# Supplementary material for: VidEoMT: Your ViT is Secretly Also a Video Segmentation Model
Source: arXiv:2602.17807 source file (2026-11-12)
Supplement: Supplementary file 3 [file failure_cases.tex]

\begin{figure*}[t]
\centering
\begin{minipage}[t]{0.45\linewidth}
    \centering
    \includegraphics[width=\linewidth]{appendix/img/failure/cavis/75a8cadb/img_0000030.jpg}
    \includegraphics[width=\linewidth]{appendix/img/failure/cavis/75a8cadb/img_0000035.jpg}
    \includegraphics[width=\linewidth]{appendix/img/failure/cavis/75a8cadb/img_0000040.jpg}
    \includegraphics[width=\linewidth]{appendix/img/failure/cavis/75a8cadb/img_0000045.jpg}
    \includegraphics[width=\linewidth]{appendix/img/failure/cavis/75a8cadb/img_0000050.jpg}
    \caption*{CAVIS (15 FPS)}
\end{minipage}
\begin{minipage}[t]{0.45\linewidth}
    \centering
    \includegraphics[width=\linewidth]{appendix/img/failure/videomt/75a8cadb/img_0000030.jpg}
    \includegraphics[width=\linewidth]{appendix/img/failure/videomt/75a8cadb/img_0000035.jpg}
    \includegraphics[width=\linewidth]{appendix/img/failure/videomt/75a8cadb/img_0000040.jpg}
    \includegraphics[width=\linewidth]{appendix/img/failure/videomt/75a8cadb/img_0000045.jpg}
    \includegraphics[width=\linewidth]{appendix/img/failure/videomt/75a8cadb/img_0000050.jpg}
    \caption*{\textbf{VidEoMT (112 FPS)}}
\end{minipage}
\caption{\textbf{Failure cases.} We illustrate failure cases of CAVIS~\citep{lee2025cavis} and VidEoMT on the OVIS dataset~\citep{qi2022occluded}. In row 3, in a highly occluded scene, identity switching occurs between persons for both models. In row 4, both methods fail to detect newly appearing elephants and persons.}
\label{app:fig:failure_case_1}
\end{figure*}

\begin{figure*}[t]
\centering
\begin{minipage}[t]{0.45\linewidth}
    \centering
    \includegraphics[width=\linewidth]{appendix/img/failure/cavis/c7b07fea/img_0000001.jpg}
    \includegraphics[width=\linewidth]{appendix/img/failure/cavis/c7b07fea/img_0000012.jpg}
    \includegraphics[width=\linewidth]{appendix/img/failure/cavis/c7b07fea/img_0000024.jpg}
    \includegraphics[width=\linewidth]{appendix/img/failure/cavis/c7b07fea/img_0000036.jpg}
    \includegraphics[width=\linewidth]{appendix/img/failure/cavis/c7b07fea/img_0000048.jpg}
    \includegraphics[width=\linewidth]{appendix/img/failure/cavis/c7b07fea/img_0000060.jpg}
    \caption*{CAVIS (15 FPS)}
\end{minipage}
\begin{minipage}[t]{0.45\linewidth}
    \centering
    \includegraphics[width=\linewidth]{appendix/img/failure/videomt/c7b07fea/img_0000001.jpg}
    \includegraphics[width=\linewidth]{appendix/img/failure/videomt/c7b07fea/img_0000012.jpg}
    \includegraphics[width=\linewidth]{appendix/img/failure/videomt/c7b07fea/img_0000024.jpg}
    \includegraphics[width=\linewidth]{appendix/img/failure/videomt/c7b07fea/img_0000036.jpg}
    \includegraphics[width=\linewidth]{appendix/img/failure/videomt/c7b07fea/img_0000048.jpg}
    \includegraphics[width=\linewidth]{appendix/img/failure/videomt/c7b07fea/img_0000060.jpg}
    \caption*{\textbf{VidEoMT (112 FPS)}}
\end{minipage}
\caption{\textbf{Failure cases.} We illustrate a failure case of CAVIS~\citep{lee2025cavis} and VidEoMT on the OVIS dataset~\citep{qi2022occluded}. Both methods fail to detect newly appearing cyclists and bicycles in later frames.}
\label{app:fig:failure_case_2}
\end{figure*}
