# Supplementary material for: VidEoMT: Your ViT is Secretly Also a Video Segmentation Model
Source: arXiv:2602.17807 source file (2026-11-12)
Supplement: Supplementary file 4 [file memory_comparsion.tex]

\definecolor{caviscolor}{HTML}{397FBE}
\definecolor{videomtcolor}{HTML}{ff6d01}
\begin{figure}[t]
\centering
\begin{tikzpicture}
\begin{axis}[
    width=0.9\linewidth,
    height=6.5cm,
    xlabel={Input Resolution (pixels)},
    ylabel={GPU Memory (GB)},
    xlabel style={font=\small\bfseries, yshift=-18pt},
    ylabel style={font=\small\bfseries},
    axis line style={thick},
    tick label style={font=\small},
    xmin=400, xmax=4200,
    ymin=0, ymax=22,
    xtick={448,1024,2048,4096},
    xticklabel style={
        rotate=40,
        anchor=north east,
        font=\small,
        /pgf/number format/set thousands separator={}
    },
    grid=major,
    grid style={dashed, gray!40},
    legend style={
        font=\small,
        at={(0.02,0.98)},
        anchor=north west,
        draw=none
    },
    enlarge x limits=0.08
]

\addplot[
    color=caviscolor,
    mark=*,
    mark size=2.8,
    line width=1.8pt
]
coordinates {
    (448,2.41)
    (1024,4.55)
    (2048,8.61)
    (4096,19.44)
};
\addlegendentry{CAVIS}

\addplot[
    color=videomtcolor,
    mark=square*,
    mark size=2.8,
    line width=1.8pt
]
coordinates {
    (448,1.74)
    (1024,2.84)
    (2048,4.92)
    (4096,9.51)
};
\addlegendentry{VidEoMT}

\end{axis}
\end{tikzpicture}
\caption{\textbf{GPU memory consumption of CAVIS and VidEoMT.} Across increasing input resolutions.}
\label{fig:memory_scaling}
\end{figure}
