# Supplementary material for: VidEoMT: Your ViT is Secretly Also a Video Segmentation Model
Source: arXiv:2602.17807 source file (2026-11-12)
Supplement: Supplementary file 7 [file model_size_app.tex]

\begin{table}[!t]
    \centering
    \footnotesize
    \renewcommand{\tabcolsep}{2.2pt}
    \begin{tabularx}{\linewidth}{l Y YYYY}

    \toprule

    Method & Size & AP & Params & GFLOPs & FPS \\

    \midrule
    
    CAVIS  && 68.9 & 358M & 838 & 15
    \\
      
    EoMT + CAVIS & L & 68.1 & 328M & 699 & 42
    \\

    \textbf{VidEoMT} & & 68.6 & 318M & 566 & 160
    \\
    
    \midrule

    CAVIS &  & 59.5 & 131M & 390 & 18
    \\ 
    EoMT + CAVIS & B & 57.4& 103M & 284 & 67
    \\

    \textbf{VidEoMT} & & 58.2 & 95M & 182 & 251
    \\

    \midrule

    CAVIS  & & 55.5 & 57M & 251 & 19
    \\
    EoMT + CAVIS & S & 50.3 & 34M & 150 & 93
    \\
    
    \textbf{VidEoMT} & & 52.8 & 25M & 56 & 294
    \\

    \bottomrule
        
    \end{tabularx}
    \caption{\textbf{Impact of model size.} VidEoMT performs better as ViT~\cite{dosovitskiy2021vit} size increases. Evaluated on YouTube-VIS 2019 \textit{val}.} 
    \label{app:tab:model_size}
\end{table}
